# Supplementary material for: High-performance matrix-free unfitted finite element operator evaluation
Source: arXiv:2404.07911 ancillary file (2024-04-12)
Supplement: Supplementary file 1 [file ex_supplement.pdf]

# SUPPLEMENTARY MATERIALS: HIGH-PERFORMANCE MATRIX-FREE UNFITTED FINITE ELEMENT OPERATOR EVALUATION*

MAXIMILIAN BERGBAUER†, PETER MUNCH‡, WOLFGANG A. WALL†, AND MARTIN KRONBICHLER §

## SM1. Ghost penalty stabilization.

**SM1.1. Volume-based stabilization.** In Figure SM1 the two different strategies for volume ghost penalty stabilization are visualized.

**SM1.2. Face-based stabilization.** For face-based ghost penalty, the additional term reads

$$g_{\mathrm{f}}(v,u) = \sum_{j=0}^{k} \tau_{\mathrm{f},j} h^{2j+1} \left( [\![\partial_n^j v]\!], [\![\partial_n^j u]\!] \right)_{\Gamma_h^{\mathrm{stab}}} \tag{SM1.1}$$

with $\partial_n^j(\cdot)$ the $j$th normal derivative, penalizing the normal derivative jumps up to order $p$ of the shape functions and $\tau_{\mathrm{f},j}$, a penalty parameter for the $j$th normal derivative. Typically, all faces on cut cells that are either intersected or on the inside of the computational domain need to be stabilized, see Figure SM2. The face-based ghost penalty stabilization is evaluated on the whole face even if the face is cut, meaning we always use structured quadrature for the additional integral.

The face-based ghost penalty (SM1.1) consists of face integrals of normal derivatives on the standard structured quadrature on the face. The matrix-free implementation for up to second-order derivatives is straightforward, as it is already available in standard (fitted) FEM codes like deal.II. Higher-order normal derivatives would also be necessary for higher-order methods ($p \geq 3$).

**SM2. Multigrid preconditioner.** In Figure SM3 the multigrid v-cycle is visualized with the chosen transfers, smoothers, and the coarse grid solver. Relevant parameters for the Chebyshev smoother with additive Schwarz preconditioner are listed in Table SM1. Smoothing is applied symmetrically as indicated in SM3. To determine the largest eigenvalue of the preconditioned system Lanczos iterations are performed. The smallest eigenvalue for the target smoothing range is determined by the *smoothing range* parameter.

**SM3. Estimates arithmetic and memory costs.** The following tables present estimated memory and arithmetic characteristics of sparse matrix, structured, and unstructured algorithms after the formulas introduced in this work.

**SM4. Roofline and throughput on different hardware.** We show the benchmark results (roofline, see Figure SM4 and throughput, see Figure SM5) also for different hardware, here Intel Xeon Gold 6230.

---

*Submitted to the editors April 11, 2024.

**Funding:** We gratefully acknowledge the support from the German Research Foundation (DFG) under the project "High-Performance Cut Discontinuous Galerkin Methods for Flow Problems and Surface-Coupled Multiphysics Problems" Grant Agreement No. 456365667.

†Technical University of Munich (maximilian.bergbauer@tum.de, wolfgang.a.wall@tum.de).

‡Uppsala University, University of Augsburg (peter.munch@it.uu.se)

§Ruhr University Bochum, University of Augsburg (martin.kronbichler@rub.de).

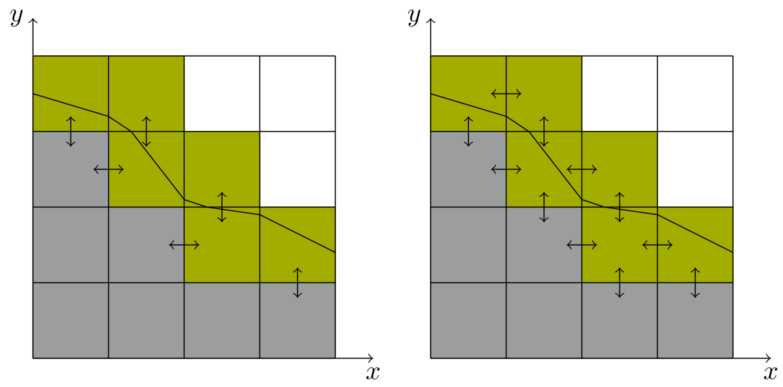


Fig. SM1: Volume-based ghost penalty: stable neighbor and all neighbors strategy, inside cells (gray) and cut cells (green)

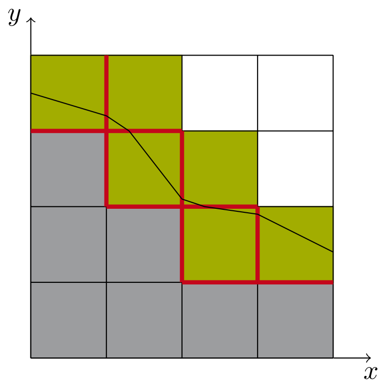


Fig. SM2: Face-based ghost penalty: inside cells (gray), cut cells (green), outside cells (white) and stabilized faces (red)

**SM5. Hardware specifications.** We present the hardware specifications of the used configurations in Table SM8.

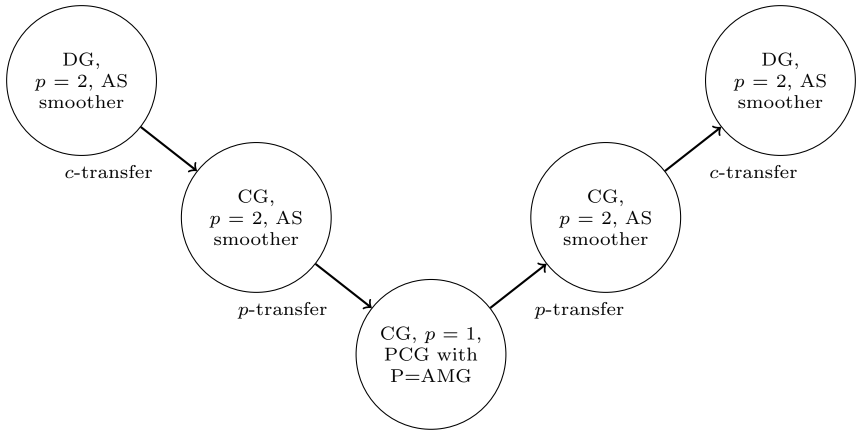


Fig. SM3: Hybrid *cp*-multigrid v-cycle preconditioner for a DG discretization with $p = 2$. A Chebyshev smoother with an additive Schwarz (AS) preconditioner is applied on each level. On the coarse level a preconditioned conjugate gradient (PCG) solver is employed with algebraic multigrid (AMG) as a preconditioner (P).

Table SM1: Smoother parameters

| smoother iterations | smoothing range | iterations eigenvalue estimation |
|---|---|---|
| 10 | 20 | 10 |

Table SM2: CG, 3D, sparse matrix

| | 1 | 2 | 3 | 4 |
|---|---|---|---|---|
| Byte/DoF | 324 | 768 | 1500 | 2592 |
| FLOPs/DoF | 54 | 128 | 250 | 432 |

Table SM3: CG, 3D, unstructured quadrature algorithm, $n_{\text{lanes}} = 8$

| | 1 | 2 | 3 | 4 |
|---|---|---|---|---|
| Byte/DoF | 339 | 169 | 110 | 96.2 |
| FLOPs/DoF evaluation/integration | 1,150 | 1,490 | 1,820 | 2,760 |
| FLOPs/DoF quadrature point | 72 | 36 | 21.3 | 18 |
| FLOPs/DoF 1D shapes | 12 | 4.5 | 2.67 | 1.88 |
| FLOPs/DoF | 1,240 | 1,530 | 1,840 | 2,780 |

Table SM4: CG, 3D, structured quadrature algorithm, $n_{\text{lanes}} = 8$

| | 1 | 2 | 3 | 4 |
|---|---|---|---|---|
| Byte/DoF | 57.8 | 37.7 | 33.5 | 31.8 |
| FLOPs/DoF evaluation/integration | 192 | 122 | 114 | 117 |
| FLOPs/DoF quadrature point | 72 | 30.4 | 21.3 | 17.6 |
| FLOPs/DoF | 264 | 152 | 135 | 135 |

Table SM5: DG, 3D, sparse matrix

| | 1 | 2 | 3 | 4 |
|---|---|---|---|---|
| Byte/DoF | 672 | 2268 | 5376 | 10500 |
| FLOPs/DoF | 112 | 378 | 896 | 1750 |

Table SM6: DG, 3D, unstructured quadrature algorithm, $n_{\text{lanes}} = 8$

| | 1 | 2 | 3 | 4 |
|---|---|---|---|---|
| Byte/DoF | 227 | 155 | 95.3 | 95.3 |
| FLOPs/DoF evaluation/integration | 648 | 1,020 | 1,180 | 2,020 |
| FLOPs/DoF quadrature point | 138 | 87.1 | 41.2 | 42.2 |
| FLOPs/DoF 1D shapes | 1.5 | 1.33 | 1.12 | 0.96 |
| FLOPs/DoF | 788 | 1,110 | 1,220 | 2,060 |

Table SM7: DG, 3D, structured quadrature algorithm, $n_{\text{lanes}} = 8$

| | 1 | 2 | 3 | 4 |
|---|---|---|---|---|
| Byte/DoF | 28.9 | 25.5 | 24.6 | 24.3 |
| FLOPs/DoF evaluation/integration | 120 | 132 | 144 | 156 |
| FLOPs/DoF quadrature point | 73.5 | 52 | 41.2 | 34.8 |
| FLOPs/DoF | 194 | 184 | 185 | 191 |

Table SM8: Hardware specifications

| | AMD EPYC 9354 | Intel Xeon Gold 6230 |
|---|---|---|
| cores | 2×32 | 2×20 |
| frequency | 3.25 GHz | 2.1 GHz |
| SIMD width & unit | 512 bit, 1 units | 512 bit, 2 units |
| peak performance (FP64) | 3200 GFlop/s | 2500 GFlop/s |
| memory interface | DDR5-4800, 24 chan. | DDR4-2933, 12 chan. |
| L3 cache | 2×256 MB | 2×27.5 MB |
| LOAD memory bandwidth | 680 GB/s | 230 GB/s |
| STREAM memory bandwidth | 500 GB/s | 125 GB/s |

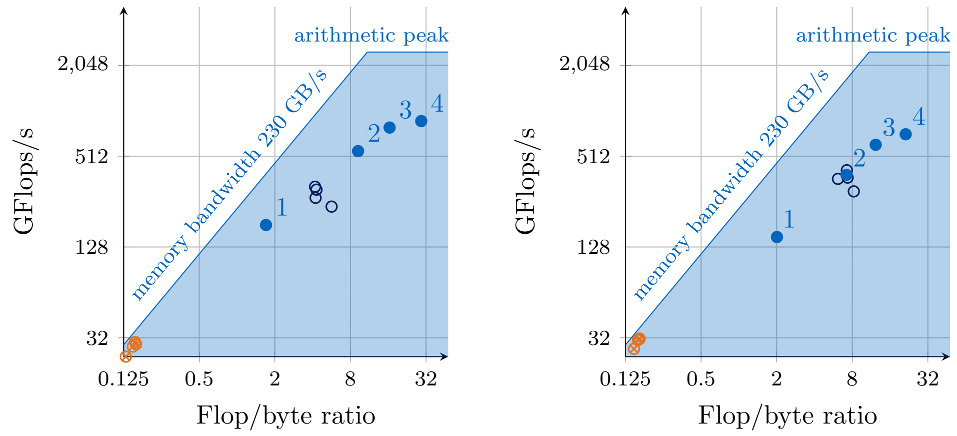


(a) CG (b) DG

Fig. SM4: Roofline performance model: 3D, classification of sparse matrix (⊗) compared to structured quadrature algorithm (○) and unstructured quadrature algorithm (●) for $p = 1, 2, 3, 4$ on Intel Xeon Gold 6230

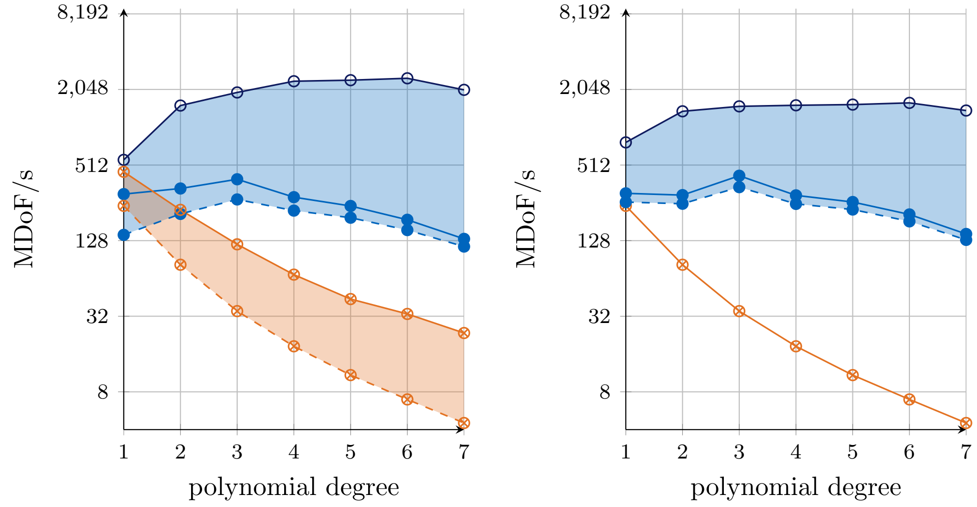


(a) CG (b) DG

Fig. SM5: Throughput: 3D, sparse matrix upper bound (—⊗—) and sparse matrix lower bound (- ⊗ -) enclosing the sparse matrix range (▭) compared to structured quadrature algorithm (—○—), unstructured quadrature algorithm with standard terms (—●—) and with additional surface terms (- ● -) enclosing the matrix-free range (▭) for $p = 1, ..., 7$ on Intel Xeon Gold 6230
